# Supplementary material for: Where is the answer? Investigating Positional Bias in Language Model Knowledge Extraction
Source: arXiv:2402.12170 source file (2025-04-18)
Supplement: Supplementary file 1 [file paper_abst_appendix.tex]

\begin{table}[h!]
\centering

\newcolumntype{Y}{>{\raggedright\arraybackslash}X}
\scalebox{0.9}{
\begin{tabularx}{0.5\textwidth}{c|Y|Y|Y}
\toprule
Augmentation&Dataset &Number&Code\\\hline
%&Replace&13.2\rise{4.4}&11.1\rise{3.3}&22.0\rise{11.4}\\\hline
None& 18.0 & 9.9& 9.6 \\
Shuffle& 7.6& 11.6 & 5.8 \\
RTR& 19.4&11.2&12.6 \\
\bottomrule
\end{tabularx}}
\vspace{-3mm}
\caption{Results of models trained on the abstract of papers. We employ LLama-13B model for comparison. }
\label{tab:paper_abst}
\end{table}
